# Supplementary material for: GSVNet: Guided Spatially-Varying Convolution for Fast Semantic Segmentation on Video
Source: arXiv:2103.08834 source file (2021-06-08)
Supplement: Supplementary file 1 [file appendix.tex]

\definecolor{green1}{RGB}{172,255,51}
\definecolor{green2}{RGB}{31, 122, 0}
\definecolor{green3}{RGB}{14,134,43}
\definecolor{red1}{RGB}{255,100,51}
\definecolor{red2}{RGB}{255,53,51}
\definecolor{red3}{RGB}{255,199,51}
\definecolor{purple1}{RGB}{195,0,255}
%\usepgfplotslibrary{external}

%%
%% The "title" command has an optional parameter,
%% allowing the author to define a "short title" to be used in page headers.
%}

\begin{appendices}

\section{Accuracy-throughput Trade-off}
Fig.~\ref{fig:acc_speed_int5} compares the accuracy-throughput curves of the competing methods. To trade lower accuracy for higher throughput, the keyframe interval is altered from 1 to 5 for A-X39 and the two variants of our scheme\footnote{The keyframe interval 1 corresponds to image-based segmentation.}, while for the image-based methods, \textcolor{black}{the input image is downscaled by a factor of 1, 0.75, 0.6, and 0.5, followed by an interpolation of the segmentation output to the full resolution}.

Fig.~\ref{fig:keyframe_com} presents more accuracy-throughput curves by choosing BiSeNet (1.0) and SwiftNet (1.0) for keyframe segmentation. This shows that our scheme can work with these image segmentation networks under different settings to offer a wide variety of accuracy-throughput trade-offs. As mentioned in the main paper, it can readily work with any off-the-shelf image segmentation network.
    \section{More Ablation Experiments}
    \subsection{Replacing Ideal-delay Kernels with Learned Kernels.}
        Table~\ref{table:set_com} indicates that little gain can be achieved by replacing the $3 \times 3$ ideal-delay kernels with learned kernels. Our reasoning is that the same net effect may be obtained by adapting the following $1 \times 1$ dynamic convolution kernels.
    
    \subsection{Enlarging Ideal-delay Kernels.}            
        Table~\ref{table:com_kernel_size} further shows that enlarging the size of the ideal-delay kernels, equivalently allowing longer-distance spatial propagation, brings modest mIoU gain at the cost of lower throughput. For this experiment, we learn the kernels end-to-end since for the $5 \times 5$ case, \textcolor{black}{only 17 out of 25 possible ideal-delay patterns are used for initialization and for maintaining high FPS}. We attribute the result to the fact that our flow propagation network operates in the 1/8-downscaled domain (cp. Fig. 6 in the main paper). The $3 \times 3$ kernel size covers already a large enough receptive field in the full-resolution image space. 
        
    \subsection{Edge Map Analysis}
    In the main paper (Section 3.4.3 Guided Dynamic Filtering), we conjecture that the warped segmentation $\hat{S}_{t}^-$ tends to be erroneous at the object boundaries and propose to provide the edge map $E_t$ derived from $\hat{S}_{t}^-$ as the guiding signal for dynamic filtering. Fig. ~\ref{fig:edge_com} validates our conjecture by showing the high correlation between the edge map and the error map (indicating the segmentation errors on $\hat{S}_{t}^-$). 
        \begin{figure}[t]
        %\captionsetup{textfont=normalfont}
        \begin{tikzpicture}
            %\centering
            \begin{axis}[
                name=axis1,
                yshift=4.5cm,
                height=4cm,width=8.5cm,
                xlabel={Throughput (FPS)},
                ylabel={Avg. mIoU ($\%$)},
                ylabel style={at={(axis description cs:0.05,0.5)}},
                xlabel style={at={(axis description cs:0.5,0.0)}},
                xmin=30, xmax=160,
                ymin=66, ymax=76,
                line width=1.0pt,
                mark size=2.0pt,
                xtick={30, 40, 50, 60, 70, 80, 90, 100, 110, 120, 130, 140,150,160},
                xmajorgrids,
                ytick={66, 68, 70, 72, 74, 76},
                ymajorgrids,
                %legend pos=south west,
                legend style={at={(-0.125, 1.7)},anchor=north west, legend  columns =3, draw=none,cells={align=left}},
                legend cell align={left},
                %/tikz/every even column/.append style={column sep=1 cm}},
                grid style={solid, gray},
            ]
            
            \addplot[
                color=cyan,
                mark=square*,
                ]
                coordinates { (61,73.7)(98.5,72.9)(123.4,72.0)(140,71.2)(153,70.3)
                };
            \addlegendentry{Ours-BiSeNet-R18}
            \addplot[
                color=green2,
                mark=triangle,
                ]
                %coordinates {(105,69)};
                %72.7,71.7,71,70.5,70.1
                coordinates {(61,72.7)(58.8,71.7)(58.1,71)(57.4,70.5)(57.1,70.1)};
            \addlegendentry{A-X39}
            %\addplot[
            %    color=black,
            %    mark=triangle*,
            %    ]%(61,73.8)
            %coordinates{(61,68.6)(63.9,69.3)(64.6,69.3)(65.0,69.1)(65.3,68.8)};
            %\addlegendentry{A-X39}
            \addplot[
                color=black,
                mark=diamond*,
                ]%(61,73.8)
             %coordinates{(123.5,68.6)};
                coordinates {(105,69)};
            \addlegendentry{BiSeNet-X39}
            
            %ours with swnet
            \addplot[
                color=blue,
                mark=*,
                ]
                coordinates { (63.2,74.4)(100,73.6)(125,72.6)(142,71.8)(155,70.9)
                };
            \addlegendentry{Ours-SwiftNet-R18}
            \addplot[
                color=red,
                dashed,
                every mark/.append style={solid},
                mark=square,
                ]
                coordinates {(37,75.1)(61,73.8)(90,69.3)(131,68.9)};
            \addlegendentry{BiSeNet-R18}
            \addplot[
                color=purple1,
                dashed,
                every mark/.append style={solid},
                mark=o,
                ]
                %96 is not sure
                coordinates {(39.3,74.6)(63.2,74.4)(92,70.9)(134,68.7)};
            \addlegendentry{SwiftNet-R18}
            \addplot[
                color=purple2,
                every mark/.append style={solid},
                mark=x,
                ]
                coordinates {(108.7,67.3)};
            \addlegendentry{EDANet}
            \addplot[
                color=orange,
                every mark/.append style={solid},
                mark=star,
                ]
                coordinates {(123.5,68.6)};
            \addlegendentry{Fast-SCNN}
            %\addplot[
            %    color=purple2,
            %    dashed,
            %    every mark/.append style={solid},
            %    mark=diamond*,
            %    ]
            %    coordinates {};
            %\addlegendentry{ERFNet}
            
            \end{axis}
            
            \begin{axis}[
                name=axis2,
                height=4cm,width=8.5cm,
                xlabel={Throughput (FPS)},
                ylabel={Min. mIoU ($\%$)},
                ylabel style={at={(axis description cs:0.05,0.5)}},
                xlabel style={at={(axis description cs:0.5,0.0)}},
                xmin=30, xmax=160,
                ymin=66, ymax=76,
                line width=1.0pt,
                mark size=2.0pt,
                xtick={30, 40, 50, 60, 70, 80, 90, 100, 110, 120, 130, 140,150,160},
                xmajorgrids,
                ytick={66, 68, 70, 72, 74, 76},
                ymajorgrids,
                %legend pos=south west,
                legend style={at={(-0.1, 1.6)},anchor=north west, legend  columns =3, draw=none},
                %/tikz/every even column/.append style={column sep=1 cm}},
                grid style={solid, gray},
            ]
            
            \addplot[
                color=cyan,
                mark=square*,
                ]
                coordinates { (61,73.7)(98.5,72.1)(123.4,70.5)(140,68.8)(153,67.1)
                };
            %72.7,70.9,69.8,69.1,68.5
            \addplot[
                color=green2,
                mark=triangle,
                ]
                coordinates {(61,72.7)(58.8,70.9)(58.1,69.8)(57.4,69.1)(57.1,68.5)
                };
            %\addplot[
            %    color=black,
            %    mark=triangle*,
            %    ]%(61,73.8)
                %coordinates{(61,68.6)(63.9,68.6)(64.6,68.6)(65.0,68.6)(65.3,68.5)};
            \addplot[
                color=black,
                mark=diamond*,
                ]%(61,73.8)
             %coordinates{(123.5,68.6)};
                coordinates {(105,69)};
            %ours with swnet
            \addplot[
                color=blue,
                mark=*,
                ]
                coordinates { (63.2,74.4)(100,72.9)(125,70.7)(142,69.6)(155,67.7)
                };
            \addplot[
                color=red,
                dashed,
                every mark/.append style={solid},
                mark=square,
                ]
                coordinates {(37,75.1)(61,73.8)(90,69.3)(131,68.9)};
            \addplot[
                color=purple1,
                dashed,
                every mark/.append style={solid},
                mark=o,
                ]
                coordinates {(39.3,74.6)(63.2,74.4)(92,70.9)(134,68.7)};
            \addplot[
                color=purple2,
                every mark/.append style={solid},
                mark=x,
                ]
                coordinates {(108.7,67.3)};
            \addplot[
                color=orange,
                every mark/.append style={solid},
                mark=star,
                ]
                coordinates {(123.5,68.6)};
            \end{axis}
            \node [below= 1.2cm] at (axis1.south) {\MakeLabel{subb}};
            \node [below= 1.2cm] at (axis2.south) {\MakeLabel{suba}};
            
        \end{tikzpicture}
        \caption{Comparison of accuracy-throughput curves evaluated on Cityscapes validation set.
        %To explore the trade-off trend of image-based methods, we take three variants based on different input scales containing $\{1.0, 0.75, 0.6, 0.5\}$ of BiSeNet~\cite{bisenet} and SwiftNet~\cite{swiftnet} for comparison.
        The dashed lines correspond to image-based methods, where different accuracy-throughput trade-offs are achieved by adapting the input resolution with factors \{1, 0.75, 0.6, 0.5\}. EDANet, Fast-SCNN, and BiSeNet-X39 have an input scaling factor of 0.5, 1, and 0.75, respectively. The solid lines are video-based methods with a variable keyframe interval ranging from 1 to 5. For keyframe segmentation, ours-BiSeNet-R18 and ours-SwiftNet-R19 adopt BiSeNet-R18 (0.75) and SwiftNet-R18 (0.75), respectively. Likewise, A-X39 uses BiSeNet-R18 (0.75). The mIoU is evaluated at full resolution without regard to the input scaling factor.}
        \vspace{-0.5cm}
        %\captionof{figure}{First caption}
        %\captionof{figure}{Second caption}
        \label{fig:acc_speed_int5}
    \end{figure}
        \begin{figure}[t]
        %\captionsetup{textfont=normalfont}
        \begin{tikzpicture}
            %\centering
            \begin{axis}[
                name=axis1,
                yshift=4.5cm,
                height=4cm,width=8.5cm,
                xlabel={Throughput (FPS)},
                ylabel={Avg. mIoU ($\%$)},
                ylabel style={at={(axis description cs:0.05,0.5)}},
                xlabel style={at={(axis description cs:0.5,0.0)}},
                xmin=30, xmax=160,
                ymin=68, ymax=76,
                line width=1.0pt,
                mark size=2.0pt,
                xtick={30, 40, 50, 60, 70, 80, 90, 100, 110, 120, 130, 140,150,160},
                xmajorgrids,
                ytick={68, 70, 72, 74, 76},
                ymajorgrids,
                %legend pos=south west,
                legend style={at={(-0.1, 1.5)},anchor=north west, legend  columns =2, draw=none,cells={align=left}},
                legend cell align={left},
                %/tikz/every even column/.append style={column sep=1 cm}},
                grid style={solid, gray},
            ]
            
            \addplot[
                color=cyan,
                mark=square,
                dashed,
                every mark/.append style={solid},
                ]
                coordinates { (61,73.7)(98.5,72.9)(123.4,72.0)(140,71.2)(153,70.3)
                };
            \addlegendentry{Ours-BN-R18 (0.75)}
            \addplot[
                color=green2,
                mark=square,
                dashed,
                every mark/.append style={solid},
                ]
                %coordinates {(105,69)};
                %72.7,71.7,71,70.5,70.1
                coordinates {(37,75.2)(64.5,74.2)(85.4,73.2)(101,72.3)(115,71.4)};
            \addlegendentry{Ours-BN-R18 (1.0)}
            
            %ours with swnet
            \addplot[
                color=blue,
                mark=*,
                ]
                coordinates { (63.2,74.4)(100,73.6)(125,72.6)(142,71.8)(155,70.9)
                };
            \addlegendentry{Ours-SN-R18 (0.75)}
            \addplot[
                color=red,
                %dashed,
                %every mark/.append style={solid},
                mark=*,
                ]
                coordinates {(37,74.6)(64.5,74.1)(85.4,73.4)(101,72.7)(115,71.9)};
            \addlegendentry{Ours-SN-R18 (1.0)}
            \end{axis}
            
            \begin{axis}[
                name=axis2,
                height=4cm,width=8.5cm,
                xlabel={Throughput (FPS)},
                ylabel={Min. mIoU ($\%$)},
                ylabel style={at={(axis description cs:0.05,0.5)}},
                xlabel style={at={(axis description cs:0.5,0.0)}},
                xmin=30, xmax=160,
                ymin=66, ymax=76,
                line width=1.0pt,
                mark size=2.0pt,
                xtick={30, 40, 50, 60, 70, 80, 90, 100, 110, 120, 130, 140,150,160},
                xmajorgrids,
                ytick={66, 68, 70, 72, 74, 76},
                ymajorgrids,
                %legend pos=south west,
                legend style={at={(-0.1, 1.5)},anchor=north west, legend  columns =2, draw=none},
                %/tikz/every even column/.append style={column sep=1 cm}},
                grid style={solid, gray},
            ]
            
            \addplot[
                color=cyan,
                mark=square,
                dashed,
                every mark/.append style={solid},
                ]
                coordinates { (61,73.7)(98.5,72.1)(123.4,70.5)(140,68.8)(153,67.1)
                };
            \addplot[
                color=green2,
                mark=square,
                dashed,
                every mark/.append style={solid},
                ]
                %coordinates {(105,69)};
                %72.7,71.7,71,70.5,70.1
                coordinates {(37,75.2)(64.5,73.3)(85.4,71.4)(101,69.8)(115,68.0)};
            %ours with swnet
            \addplot[
                color=blue,
                mark=*,
                ]
                coordinates { (63.2,74.4)(100,72.9)(125,70.7)(142,69.6)(155,67.7)
                };
            \addplot[
                color=red,
                %dashed,
                %every mark/.append style={solid},
                mark=*,
                ]
                coordinates {(37,74.6)(64.5,73.6)(85.4,72.0)(101,70.7)(115,69.1)};
            \end{axis}
            \node [below= 1.2cm] at (axis1.south) {\MakeLabel{subb}};
            \node [below= 1.2cm] at (axis2.south) {\MakeLabel{suba}};
            
        \end{tikzpicture}
        \caption{Comparison of accuracy-throughput curves.}
        \label{fig:keyframe_com}
    \end{figure}
        \begin{table}[t]
        \centering
        \setlength{\tabcolsep}{5pt}
        %\captionsetup{textfont=normalfont}
        \begin{tabular}{p{0.2\linewidth}p{0.2\linewidth}ccccc}
            \hline
             & & \multicolumn{5}{c}{Keyframe interval} \\ \cline{3-7}
            Metric & Scheme & 1 & 2 & 3 & 4 & 5 \\ \hline
            Avg. & IDK & 74.4 & 73.7 & 72.6 & 71.8 & 70.9 \\ 
            %  & RI+TK & 74.4 & 73.6 & 72.5 & 71.6 & 70.6 \\
            mIoU ($\%$) & IDK+Finetune & 74.4 & 73.6 & 72.6 & 71.8 & 70.9 \\
            \hline
        \end{tabular}
        \vspace{0.5em}
        \caption{Accuracy comparison between models with ideal-delay kernels and fine-tuned kernels for various keyframe intervals. \textbf{IDK:} Ideal-delay Kernel.}
        \label{table:set_com}
    \end{table}
        \begin{table}[t]
        %\centering\footnotesize
        \setlength{\tabcolsep}{6pt}
        %\captionsetup{textfont=normalfont}
        \begin{tabular}{p{0.2\linewidth}p{0.2\linewidth}|ccc}
            \hline
            Kernel & $\#$ of & Avg.  & Min. & FPS \\ 
            size & filters & mIoU ($\%$) & mIoU ($\%$) \\ \hline
            3 $\times$ 3 &  9 & 70.9 & 67.7 & 155 \\
            %3 $\times$ 3 & 17 & 70.9 & 67.6 & 148 \\
            %5 $\times$ 5 &  9 & 71.0 & 67.7 & 151 \\
            5 $\times$ 5 & 17 & 71.1 & 67.9 & 144 \\
            %7 $\times$ 7 &  9 & 71.0 & 67.8 & 146 \\
            %7 $\times$ 7 & 17 & 71.1 & 68.0 & 140 \\
            \hline
        \end{tabular}
        \vspace{0.5em}
        \caption{Impact of the size of the ideal-delay kernels on accuracy and throughput. The mIoU is measured at the keyframe interval of 5.}
        \label{table:com_kernel_size}
    \end{table}
        \begin{figure}[ht]
        \centering
        %\setlength\tabcolsep{0.25em}
        %\captionsetup{textfont=normalfont}
        \begin{tabular}{@{}cc@{}}
        \includegraphics[width=4cm, height=2cm]{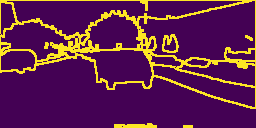} &  \includegraphics[width=4cm, height=2cm]{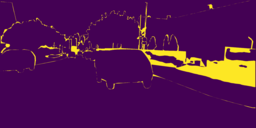}\\
           (a) Edge map & (b) Error map  \\
        \end{tabular}
        \caption{Comparison between the edge map $E_t$ and the error map, which indicates the errors on the temporally warped segmentation $\hat{S}_{t}^-$.}
        \label{fig:edge_com}
    \end{figure}
        \begin{figure}[ht]
        \centering\footnotesize
        %\captionsetup{textfont=normalfont}
        \includegraphics[height=11cm, width=.8\linewidth]{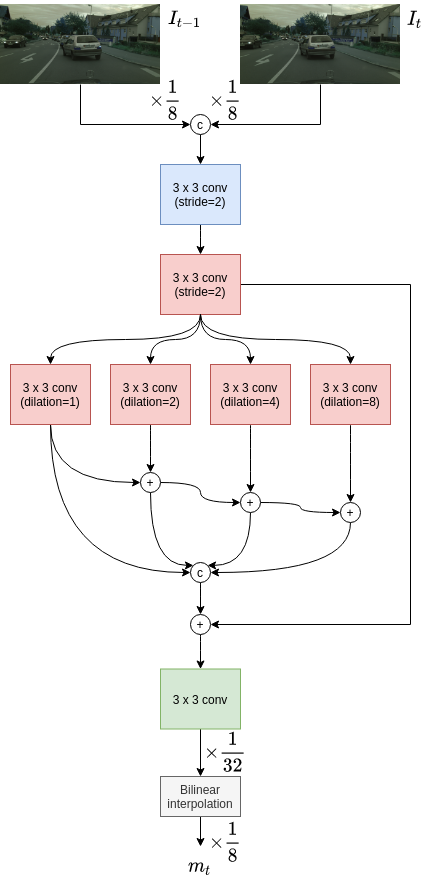}
        \vspace{-0.4cm}
        \caption{The architecture of our lightweight optical flow network. The red, blue, and green blocks each output 64, 32, and 2 channels, respectively. Except for the gray and green blocks, the other blocks all include $3 \times 3$ convolutional layers followed by batch normalization and LeakyReLU with a slope factor of 0.1.}
        \label{fig:hffb_arc}
        \vspace{-0.3cm}
    \end{figure}

\section{Lightweight Optical Flow Network}
Fig.~\ref{fig:hffb_arc} details the architecture of our lightweight optical flow network $O$. It is built based on the hierarchical feature fusion block (HFFB), initially proposed for image super resolution.
%, initially proposed in ~\cite{ppo_isr} for image super resolution. 
It first concatenates two input frames, $I_{t-1}$ and $I_{t}$, followed by passing them through two $3 \times 3$ convolutional layers with stride 2. The resulting feature maps are then input to HFFB, which consists of 4 convolutional layers with dilation 1, 2, 4, and 8. The outputs of these convolutional layers are added and pooled hierarchically as illustrated in the figure. Finally, a $3 \times 3$ convolution is applied to get a downscaled flow map $m_t$, which is interpolated bilinearly to the resolution of one-eighth of the resolution of input image.

\section{Inference Runtime}
    We apply a breakdown analysis of inference runtime on non-keyframe segmentation for A-X39 and our scheme in Fig.~\ref{fig:bk_speed}. The operation of non-keyframe segmentation is divided into four major parts: (1) optical flow estimation, (2) temporal warping in the feature or segmentation output space, (3) feature extraction from the current video frame, and (4) fusion of features or segmentation predictions. The runtimes of the three image-based methods (i.e. BiSeNet-X39, BiSeNet-R18, and SwiftNet-R18), which turn non-keyframes into keyframes for processing, are provided as monolithic quantities for comparison. 
    
    Several observations can be made from Fig.~\ref{fig:bk_speed}. First, A-X39 runs slower than all the image-based schemes, including BiSeNet-R18, i.e. the network used for keyframe segmentation in A-X39. Careful examination of A-X39 suggests that the additional operations needed for flow estimation and temporal warping outweigh its runtime reduction from the use of the lightweight feature extractor in BiSeNet-X39. This explains our earlier finding that increasing non-keyframes in A-X39 leads to a slight decrease in throughput. Second, the runtime of A-X39 is still dominated by the feature extraction from the current frame. In contrast, our lightweight flow estimation network consumes only about one-third of the runtime of FlowNet2s~\cite{flownet2s} in A-X39. Moreover, performing temporal warping in the segmentation output space (ours) consumes much less time than in the feature space (A-X39). This is because temporal warping is a memory-intensive operation. %As presented in Table \ref{table:com_warp_speed}, 
    Although the feature space in the present case has a spatial resolution (of $64 \times 128$) that is 4 times smaller than the segmentation output space (of size $128 \times 256$), it has 256/19=13.4 times more channels, thereby leading to a 3.3 times increase in data to be moved around. Third, our feature extraction from the current frame represents only a small portion of the entire inference runtime, and is much simpler than that of A-X39. The improvement comes from downscaling the input image by a factor of 1/8 and using only 3 convolutional layers for feature extraction (cp. Fig. 2 in the main paper). \textcolor{black}{Our ablation study, however, shows that without the guided dynamic filtering (Section 3.4 in the main paper), A-X39 cannot benefit from such a lightweight feature extractor. This also explains why the fusion of segmentation predictions through guided dynamic filtering constitutes a major source of complexity in our scheme}.
    
    Last but not least, the runtime distribution of our propagation framework justifies the aim of conserving computation for feature extraction from the current frame through exploiting temporal correlation between video frames.

    \begin{figure}
        \centering
        %\captionsetup{textfont=normalfont}
        \begin{tikzpicture}
        \begin{axis}[
            height=5cm,
            width=.8\linewidth,
            xbar stacked,
            xmajorgrids,
            xminorgrids,
            minor x tick num=4,
            xmin=0,
        	bar width=15pt,
        	%nodes near coords,
            %enlargelimits=0.2,
            enlarge y limits=0.2,
            legend style={at={(-0.15, 1.3)},
              anchor=north west,legend columns=2, draw=none},
            legend cell align={left},
            xlabel={Time (ms)},
            symbolic y coords={{Ours-SwiftNet-R18},A-X39,{SwiftNet-R18 (0.75)},{BiSeNet-R18 (0.75)},BiSeNet-X39},
            ytick=data,
            major grid style={solid, black},
            %y tick label style={rotate=45,anchor=east},
            ]
        \addplot+[purple2,xbar] plot coordinates {(1.1,{Ours-SwiftNet-R18})(3.8,A-X39)(0,{SwiftNet-R18 (0.75)})(0,{BiSeNet-R18 (0.75)})(0,BiSeNet-X39)};
        \addlegendentry{Flow estimation}
        \addplot+[cyan,xbar] plot coordinates {(1.0,{Ours-SwiftNet-R18})(3.3,A-X39)(0,{SwiftNet-R18 (0.75)})(0,{BiSeNet-R18 (0.75)})(0,BiSeNet-X39)};
        \addlegendentry{Temporal warping}
        \addplot+[green2,xbar] plot coordinates {(0.4,{Ours-SwiftNet-R18})(10.5,A-X39)(0,{SwiftNet-R18 (0.75)})(0,{BiSeNet-R18 (0.75)})(0,BiSeNet-X39)};
        \addlegendentry{Feature extraction}
        \addplot+[orange,xbar] plot coordinates {(1.6,{Ours-SwiftNet-R18})(0.5,A-X39)(0,{SwiftNet-R18 (0.75)})(0,{BiSeNet-R18 (0.75)})(0,BiSeNet-X39)};
        \addlegendentry{Feature/Segmentation fusion}
        %\addplot+[cyan,xbar] plot coordinates {(1.6,Ours)(0,A-X39)(0,SwiftNet)(0,BiSeNet-R18)};
        %\addlegendentry{Segmentation fusion}
        \addplot+[white,xbar,            postaction={
            pattern=crosshatch dots
        }] plot coordinates {(0,{Ours-SwiftNet-R18})(0,A-X39)(15.2,{SwiftNet-R18 (0.75)})(0,{BiSeNet-R18 (0.75)})(0,BiSeNet-X39)};
        %\addlegendentry{SwiftNet}
        \addplot+[white,xbar,postaction={
            pattern=crosshatch dots
        }] plot coordinates {(0,{Ours-SwiftNet-R18})(0,A-X39)(0,{SwiftNet-R18 (0.75)})(16,{BiSeNet-R18 (0.75)})(0,BiSeNet-X39)};
        \addplot+[white,xbar,postaction={
            pattern=crosshatch dots
        }] plot coordinates {(0,{Ours-SwiftNet-R18})(0,A-X39)(0,{SwiftNet-R18 (0.75)})(0,{BiSeNet-R18 (0.75)})(11,BiSeNet-X39)};
        %\addlegendentry{BiSeNet-R18}
        
        %\legend{\strut Flow network, \strut Warping}
        \end{axis}
        \end{tikzpicture}
        \caption{A breakdown analysis of inference runtime.}
        \label{fig:bk_speed}
    \end{figure}

\end{appendices}
